# Supplementary material for: UrduBench: An Urdu Reasoning Benchmark using Contextually Ensembled Translations with Human-in-the-Loop
Source: arXiv:2601.21000 source file (2026-01-28)
Supplement: Supplementary file 2 [file ubench_appendix_table_2.pdf]

| Marking Criteria | Evaluation Question | Correct Example | Incorrect Example |
| --- | --- | --- | --- |
| **1. Response Completeness** | Does the translation fully capture the source text without omitting any part? | **Original:** The cat sat on the mat.<br>**Translation:** بلی چٹائی پر بیٹھی تھی۔ | **Original:** The cat sat on the mat.<br>**Translation 1:** بلی بیٹھی تھی۔ (Omitting “on the mat”)<br>**Translation 2:** I don’t know (No response) |
| **2. Translation vs Generation** | Is the output a translation and not new content generation? | **Original:** The boy reads a book.<br>**Translation:** لڑکا کتاب پڑھتا ہے۔ | **Original:** The boy reads a book.<br>**Translation:** لڑکا کتاب کے بارے میں سوچتا ہے۔ (New content generated) |
| **3. Grammar and Structure** | Is the grammar and structure of the Urdu translation accurate? | **Original:** She went to the market.<br>**Translation:** وہ بازار گئی۔<br>**Original:** I bought an iPhone today.<br>**Translation:**<br>میں نے آج ایک iPhone خریدا۔ | **Original:** She went to the market.<br>**Translation:** وہ بازار گیا۔ (Incorrect gender agreement)<br>**Original:** I bought an iPhone today.<br>**Translation:** خریدا میں نے آج ایک iphone- (Incorrect placement of English equivalent) |
| **4. Number and Date Formats** | Are the number and date formats preserved as in the original? | **Original:** The event is on 12/12/2024.<br>**Translation:** یہ تقریب 12/12/2024 کو ہے | **Original:** The event is on 12/12/2024.<br>**Translation:** یہ تقریب ۱۲/۱۲/۲۰۲۴ کو ہے۔ (Converted to Arabic numerals) |
| **5. Cultural Considerations** | Are idioms translated using cultural equivalents, not literal translations? | **Original:** The ball is in your court.<br>**Translation:** فیصلہ اب آپ کے ہاتھ میں ہے۔ (Cultural equivalent used) | **Original:** The ball is in your court.<br>**Translation:** گیند اب آپ کے کورٹ میں ہے۔ (Literal translation) |
| **6. Common Error Patterns** | Does the translation avoid direct transliteration and ensure meaningful translation? | **Original:** He is an experienced teacher.<br>**Translation:** وہ تجربہ کار استاد ہے۔ | **Original:** He is an experienced teacher.<br>**Translation:** وہ ایک ایکسپرینسڈ ٹیچر ہے۔ (Direct transliteration) |
| **7. Style and Register** | Is the translation’s tone and formality consistent with the source text? | **Original:** Please submit your documents at the earliest convenience.<br>**Translation:** براہ کرم اپنی دستاویزات جلد از جلد جمع کرائیں۔ | **Original:** Please submit your documents at the earliest convenience.<br>**Translation:** دستاویزات دے دیں۔ (Casual tone used instead of formal |
