# Supplementary material for: UrduBench: An Urdu Reasoning Benchmark using Contextually Ensembled Translations with Human-in-the-Loop
Source: arXiv:2601.21000 source file (2026-01-28)
Supplement: Supplementary file 3 [file Copy_of_ubench_appendix_table_1__1_.pdf]

| English question with choices                                                                                                                                                                                                                                                                                                                          | Translation without Context                                                                                                                                                                                                                                                                                                                                          | Context Aware Translation<br>(with human validation)                                                                                                                                                                                                                                                                                                            |
|--------------------------------------------------------------------------------------------------------------------------------------------------------------------------------------------------------------------------------------------------------------------------------------------------------------------------------------------------------|----------------------------------------------------------------------------------------------------------------------------------------------------------------------------------------------------------------------------------------------------------------------------------------------------------------------------------------------------------------------|-----------------------------------------------------------------------------------------------------------------------------------------------------------------------------------------------------------------------------------------------------------------------------------------------------------------------------------------------------------------|
| <p><b>The sun is responsible for:</b></p> <p>a. puppies learning new tricks</p> <p>b. children growing up and getting old</p> <p>c. flowers wilting in a vase</p> <p>d. plants sprouting, blooming and wilting</p>                                                                                                                                     | <p>سورج ذمے دار ہے:</p> <p>a. کتنے کے بچوں نے تربیت سیکھ رہے ہیں</p> <p>b. بچے بڑے ہو رہے ہیں اور بوڑھے ہو رہے ہیں</p> <p>c. گلدان میں پھول مر جھا رہے ہیں</p> <p>d. پودے آگ رہے ہیں، پھل رہے ہیں اور مر جھا رہے ہیں</p>                                                                                                                                             | <p>سورج ذمے دار ہے:</p> <p>a. کتنے کے بچوں کے ننہ کی تربیت سیکھنے کا</p> <p>b. بچوں کے بڑے ہونے اور بوڑھے ہونے کا</p> <p>c. گلدان میں پھولوں کے مر جھانے کا</p> <p>d. پودوں کے اگنے، کھلنے اور مر جھانے کا</p>                                                                                                                                                  |
| <p><b>Squirrels spend their fall:</b></p> <p>a. looking for pretty leaves to collect</p> <p>b. stockpiling rocks for fighting in the winter</p> <p>c. stockpiling pecans for the frigid months</p> <p>d. collecting twigs to keep warm</p>                                                                                                             | <p>گھریاں خزاں کا موسم گزارتی ہیں:</p> <p>a. جمع کرنے کے لیے خوبصورت پتے تلاش کر رہی ہیں</p> <p>b. موسم سرما میں اڑنے کے لیے پرندوں کا ذخیرہ کرنا</p> <p>c. شدید سردی کے مہینوں کے لیے لیندھن کا ذخیرہ کرنا</p> <p>d. گرم رکھنے کے لیے تہہ دار لباس جمع کرنا</p>                                                                                                     | <p>گھریاں خزاں کا موسم گزارتی ہیں:</p> <p>a. خوبصورت پتے جمع کرتے ہوئے</p> <p>b. سردیوں میں لڑائی کے لیے پتھر ذخیرہ کرتے ہوئے</p> <p>c. شدید سردی کے مہینوں کے لیے پیکن ذخیرہ کرتے ہوئے</p> <p>d. گرم رہنے کے لیے ٹہنیاں جمع کرتے ہوئے</p>                                                                                                                      |
| <p><b>Sean was in a rush to get home, but the light turned yellow and he was forced to do what?</b></p> <p>a. take time</p> <p>b. dawdle</p> <p>c. go slowly</p> <p>d. ocean</p> <p>e. slow down</p>                                                                                                                                                   | <p>شان کو گھر پہنچنے کی جلدی تھی، لیکن ٹریفک سگنل کی بتی پیلی ہو گئی اور وہ کس چیز پر مجبور ہو گیا؟</p> <p>a. وقت ضائع کرنا</p> <p>b. ٹال مٹول کرنا</p> <p>c. ڈھیل ڈالنا</p> <p>d. سمندر</p> <p>e. آہستہ چلو</p>                                                                                                                                                     | <p>شان کو گھر پہنچنے کی جلدی تھی، لیکن ٹریفک سگنل کی بتی پیلی ہو گئی اور وہ کس چیز پر مجبور ہو گیا؟</p> <p>a. وقت لینا</p> <p>b. وقت ضائع کرنا</p> <p>c. رفتار آہستہ کرنے پر</p> <p>d. سمندر</p> <p>e. رفتار کم کرنا</p>                                                                                                                                        |
| <p><b>The runner was in third place, but he pushed harder and thought he might be able to reach second. What was beginning to do?</b></p> <p>a. near finish line</p> <p>b. finish</p> <p>c. get tired</p> <p>d. gain ground</p> <p>e. trip over</p>                                                                                                    | <p>وہ رنر تیسرے نمبر پر تھا، لیکن اُس نے اور زور لگایا اور سوچا کہ وہ شاید دوسرے نمبر پر پہنچ سکے۔ وہ کیا کرنے لگا تھا؟</p> <p>a. خطِ اختتام کے قریب</p> <p>b. ختم کرو / مکمل کرو</p> <p>c. تھک جانا</p> <p>d. مقبول ہونا</p> <p>e. ٹھوکر کھانا</p>                                                                                                                  | <p>وہ رنر تیسرے نمبر پر تھا، لیکن اُس نے اور زور لگایا اور سوچا کہ وہ شاید دوسرے نمبر پر پہنچ سکے۔ وہ کیا کرنے لگا تھا؟</p> <p>a. اختتامی لکیر کے قریب پہنچنا</p> <p>b. ختم کرنا</p> <p>c. تھک جانا</p> <p>d. سبقت لے جانا</p> <p>e. ٹھوکر کھانا</p>                                                                                                            |
| <p><b>A person wants to start saving money so that they can afford a nice vacation at the end of the year. After looking over their budget and expenses, they decide the best way to save money is to</b></p> <p>a. make more phone calls</p> <p>b. quit eating lunch out</p> <p>c. buy less with monopoly money</p> <p>d. have lunch with friends</p> | <p>ایک شخص سال کے آخر میں ایک اچھی چھٹی گزارنے کے لیے پیسے بچانا شروع کرنا چاہتا ہے۔ اپنے بجٹ اور اخراجات کا جائزہ لینے کے بعد، وہ فیصلہ کرتا ہے کہ پیسے بچانے کا بہترین طریقہ یہ ہے کہ</p> <p>a. زیادہ فون کا لڑ کر د</p> <p>b. باہر دوپہر کا کھانا کھانا چھوڑ دینا</p> <p>c. مونوپولی کے پیسوں سے کم خریداری کریں</p> <p>d. دوستوں کے ساتھ دوپہر کا کھانا کھاد</p> | <p>ایک شخص سال کے آخر میں ایک اچھی چھٹی گزارنے کے لیے پیسے بچانا شروع کرنا چاہتا ہے۔ اپنے بجٹ اور اخراجات کا جائزہ لینے کے بعد، وہ فیصلہ کرتا ہے کہ پیسے بچانے کا بہترین طریقہ یہ ہے کہ</p> <p>a. زیادہ فون کا لڑ کریں</p> <p>b. باہر دوپہر کا کھانا کھانا چھوڑ دیں</p> <p>c. مونوپولی کے پیسوں سے کم خریدیں</p> <p>d. دوستوں کے ساتھ دوپہر کا کھانا کھائیں</p> |
